# Supplementary material for: Few-shot Object Grounding and Mapping for Natural Language Robot Instruction Following
Source: arXiv:2011.07384 source file (2020-11-14)
Supplement: Supplementary file 1 [file app_discriminator.tex]

\begin{figure}
\centering
\includegraphics[scale=0.4]{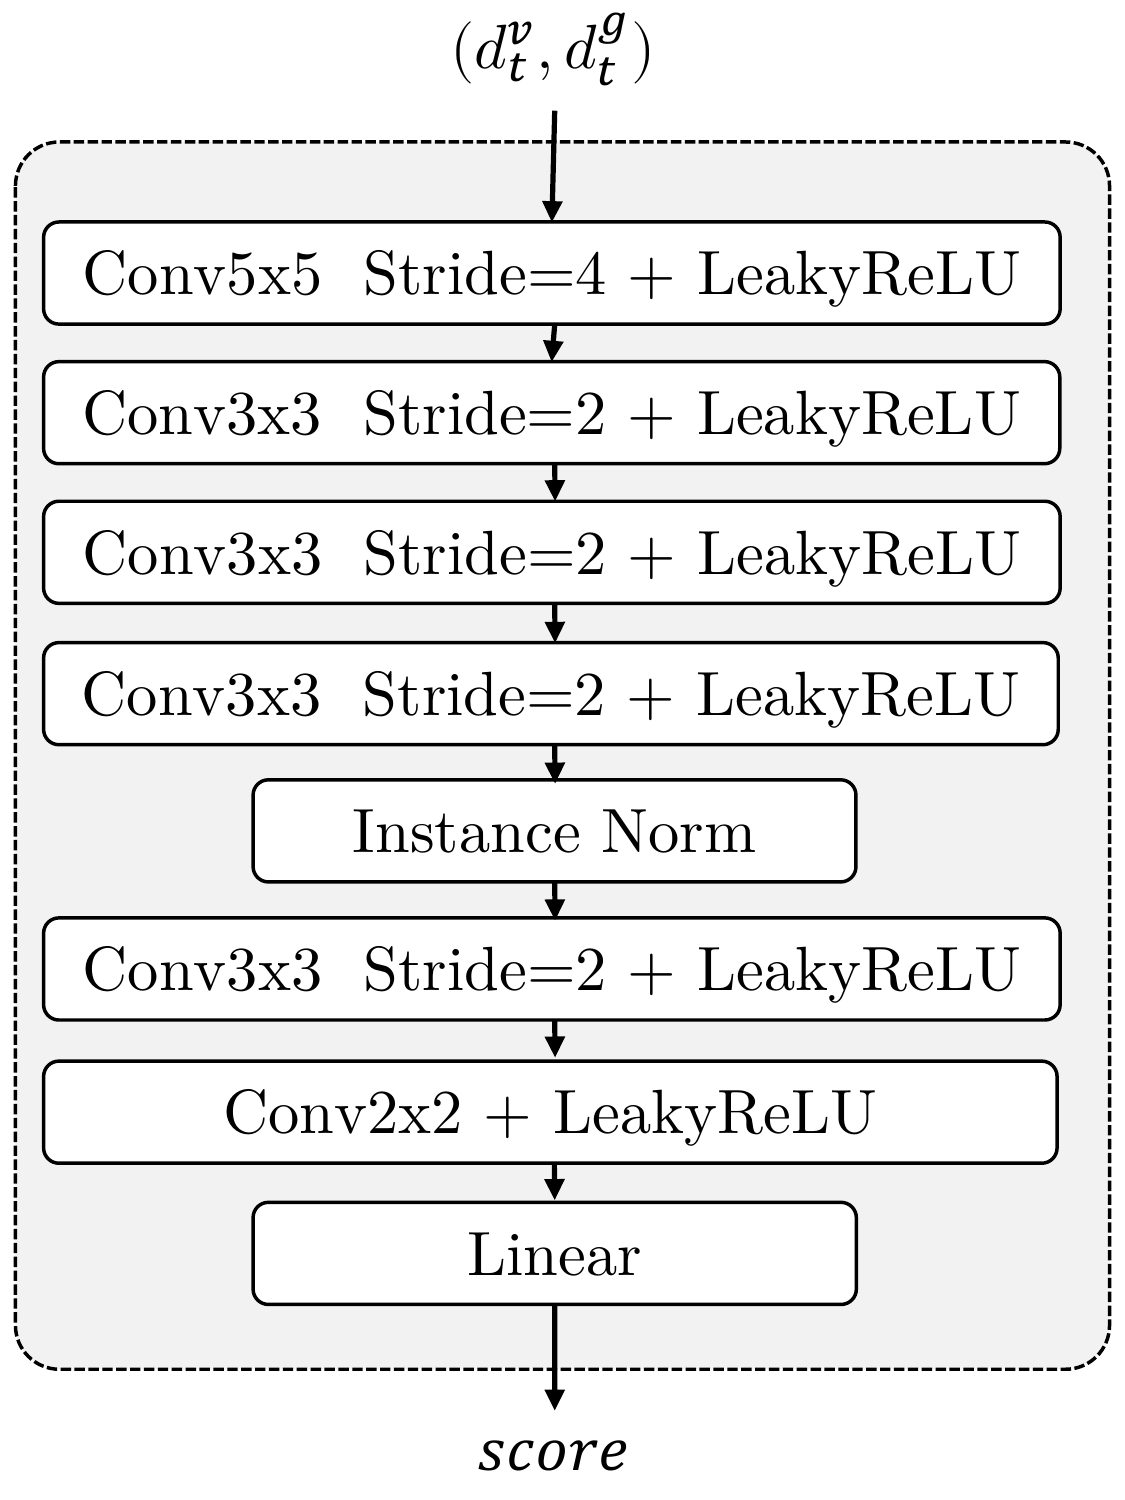}
\caption{Visitation distribution discriminator architecture.}
\label{fig:discriminator}
\end{figure}
